# Supplementary material for: EncQA: Benchmarking Vision-Language Models on Visual Encodings for Charts
Source: arXiv:2508.04650 source file (2025-08-06)
Supplement: Supplementary file 1 [file appendix_a.tex]

\begin{landscape}
\thispagestyle{empty} 

\begin{table}
\caption{\eqa{} accuracy ($\pm$ half-width of 95\% confidence interval) for all models in our evaluation suite.}
\label{tab:big_table_appendix}
\begin{tabular}{llccccccccc}
\toprule
\textbf{Task} & \textbf{Encoding} & \makecell[c]{GPT-4o} & \makecell[c]{GPT-4o mini} & \makecell[c]{o1} & \makecell[c]{InternVL2 26B} & \makecell[c]{InternVL2 8B} & \makecell[c]{InternVL2 2B} & \makecell[c]{Phi-3.5} & \makecell[c]{Molmo-7B-D} & \makecell[c]{ChartGemma} \\
\midrule
\midrule
\multirow{0}{*}{\makecell[l]{Retrieve Value }}& Length & 0.38\,{\color{darkgray}\footnotesize$\pm$\,0.11} & 0.20\,{\color{darkgray}\footnotesize$\pm$\,0.11} & 0.34\,{\color{darkgray}\footnotesize$\pm$\,0.12} & 0.72\,{\color{darkgray}\footnotesize$\pm$\,0.15} & 0.66\,{\color{darkgray}\footnotesize$\pm$\,0.13} & 0.72\,{\color{darkgray}\footnotesize$\pm$\,0.13} & 0.64\,{\color{darkgray}\footnotesize$\pm$\,0.12} & 0.64\,{\color{darkgray}\footnotesize$\pm$\,0.16} & 0.62\,{\color{darkgray}\footnotesize$\pm$\,0.14} \\
& Position & 0.54\,{\color{darkgray}\footnotesize$\pm$\,0.13} & 0.26\,{\color{darkgray}\footnotesize$\pm$\,0.11} & 0.48\,{\color{darkgray}\footnotesize$\pm$\,0.15} & 0.48\,{\color{darkgray}\footnotesize$\pm$\,0.12} & 0.56\,{\color{darkgray}\footnotesize$\pm$\,0.10} & 0.54\,{\color{darkgray}\footnotesize$\pm$\,0.13} & 0.72\,{\color{darkgray}\footnotesize$\pm$\,0.13} & 0.60\,{\color{darkgray}\footnotesize$\pm$\,0.12} & 0.62\,{\color{darkgray}\footnotesize$\pm$\,0.11} \\
& Area & 0.20\,{\color{darkgray}\footnotesize$\pm$\,0.11} & 0.20\,{\color{darkgray}\footnotesize$\pm$\,0.10} & 0.14\,{\color{darkgray}\footnotesize$\pm$\,0.08} & 0.10\,{\color{darkgray}\footnotesize$\pm$\,0.10} & 0.06\,{\color{darkgray}\footnotesize$\pm$\,0.06} & 0.14\,{\color{darkgray}\footnotesize$\pm$\,0.09} & 0.12\,{\color{darkgray}\footnotesize$\pm$\,0.08} & 0.08\,{\color{darkgray}\footnotesize$\pm$\,0.07} & 0.02\,{\color{darkgray}\footnotesize$\pm$\,0.03} \\
& Color Quantitative & 0.16\,{\color{darkgray}\footnotesize$\pm$\,0.14} & 0.04\,{\color{darkgray}\footnotesize$\pm$\,0.06} & 0.16\,{\color{darkgray}\footnotesize$\pm$\,0.14} & 0.00\,{\color{darkgray}\footnotesize$\pm$\,0.00} & 0.04\,{\color{darkgray}\footnotesize$\pm$\,0.06} & 0.00\,{\color{darkgray}\footnotesize$\pm$\,0.00} & 0.04\,{\color{darkgray}\footnotesize$\pm$\,0.06} & 0.04\,{\color{darkgray}\footnotesize$\pm$\,0.06} & 0.04\,{\color{darkgray}\footnotesize$\pm$\,0.04} \\
& Color Nominal & 0.96\,{\color{darkgray}\footnotesize$\pm$\,0.06} & 0.56\,{\color{darkgray}\footnotesize$\pm$\,0.16} & 0.76\,{\color{darkgray}\footnotesize$\pm$\,0.16} & 0.56\,{\color{darkgray}\footnotesize$\pm$\,0.17} & 0.84\,{\color{darkgray}\footnotesize$\pm$\,0.14} & 0.20\,{\color{darkgray}\footnotesize$\pm$\,0.14} & 0.84\,{\color{darkgray}\footnotesize$\pm$\,0.17} & 0.92\,{\color{darkgray}\footnotesize$\pm$\,0.10} & 0.04\,{\color{darkgray}\footnotesize$\pm$\,0.04} \\
& Shape & 0.96\,{\color{darkgray}\footnotesize$\pm$\,0.06} & 0.44\,{\color{darkgray}\footnotesize$\pm$\,0.12} & 0.80\,{\color{darkgray}\footnotesize$\pm$\,0.12} & 0.48\,{\color{darkgray}\footnotesize$\pm$\,0.16} & 0.28\,{\color{darkgray}\footnotesize$\pm$\,0.20} & 0.24\,{\color{darkgray}\footnotesize$\pm$\,0.16} & 0.64\,{\color{darkgray}\footnotesize$\pm$\,0.17} & 0.88\,{\color{darkgray}\footnotesize$\pm$\,0.13} & 0.00\,{\color{darkgray}\footnotesize$\pm$\,0.00} \\
\midrule
\multirow{0}{*}{\makecell[l]{Filter Values }}& Length & 0.91\,{\color{darkgray}\footnotesize$\pm$\,0.05} & 0.52\,{\color{darkgray}\footnotesize$\pm$\,0.10} & 0.79\,{\color{darkgray}\footnotesize$\pm$\,0.06} & 0.79\,{\color{darkgray}\footnotesize$\pm$\,0.08} & 0.62\,{\color{darkgray}\footnotesize$\pm$\,0.11} & 0.06\,{\color{darkgray}\footnotesize$\pm$\,0.05} & 0.59\,{\color{darkgray}\footnotesize$\pm$\,0.07} & 0.44\,{\color{darkgray}\footnotesize$\pm$\,0.09} & 0.05\,{\color{darkgray}\footnotesize$\pm$\,0.04} \\
& Position & 0.84\,{\color{darkgray}\footnotesize$\pm$\,0.06} & 0.41\,{\color{darkgray}\footnotesize$\pm$\,0.09} & 0.91\,{\color{darkgray}\footnotesize$\pm$\,0.04} & 0.41\,{\color{darkgray}\footnotesize$\pm$\,0.07} & 0.21\,{\color{darkgray}\footnotesize$\pm$\,0.08} & 0.03\,{\color{darkgray}\footnotesize$\pm$\,0.03} & 0.33\,{\color{darkgray}\footnotesize$\pm$\,0.10} & 0.26\,{\color{darkgray}\footnotesize$\pm$\,0.09} & 0.06\,{\color{darkgray}\footnotesize$\pm$\,0.03} \\
& Area & 0.79\,{\color{darkgray}\footnotesize$\pm$\,0.06} & 0.36\,{\color{darkgray}\footnotesize$\pm$\,0.07} & 0.62\,{\color{darkgray}\footnotesize$\pm$\,0.09} & 0.34\,{\color{darkgray}\footnotesize$\pm$\,0.07} & 0.20\,{\color{darkgray}\footnotesize$\pm$\,0.07} & 0.01\,{\color{darkgray}\footnotesize$\pm$\,0.01} & 0.12\,{\color{darkgray}\footnotesize$\pm$\,0.06} & 0.05\,{\color{darkgray}\footnotesize$\pm$\,0.04} & 0.05\,{\color{darkgray}\footnotesize$\pm$\,0.04} \\
& Color Quantitative & 0.76\,{\color{darkgray}\footnotesize$\pm$\,0.11} & 0.36\,{\color{darkgray}\footnotesize$\pm$\,0.10} & 0.60\,{\color{darkgray}\footnotesize$\pm$\,0.14} & 0.10\,{\color{darkgray}\footnotesize$\pm$\,0.08} & 0.16\,{\color{darkgray}\footnotesize$\pm$\,0.11} & 0.00\,{\color{darkgray}\footnotesize$\pm$\,0.00} & 0.14\,{\color{darkgray}\footnotesize$\pm$\,0.10} & 0.22\,{\color{darkgray}\footnotesize$\pm$\,0.10} & 0.04\,{\color{darkgray}\footnotesize$\pm$\,0.05} \\
& Color Nominal & 0.26\,{\color{darkgray}\footnotesize$\pm$\,0.13} & 0.20\,{\color{darkgray}\footnotesize$\pm$\,0.12} & 0.52\,{\color{darkgray}\footnotesize$\pm$\,0.13} & 0.08\,{\color{darkgray}\footnotesize$\pm$\,0.06} & 0.08\,{\color{darkgray}\footnotesize$\pm$\,0.06} & 0.02\,{\color{darkgray}\footnotesize$\pm$\,0.02} & 0.32\,{\color{darkgray}\footnotesize$\pm$\,0.12} & 0.08\,{\color{darkgray}\footnotesize$\pm$\,0.08} & 0.00\,{\color{darkgray}\footnotesize$\pm$\,0.00} \\
& Shape & 0.50\,{\color{darkgray}\footnotesize$\pm$\,0.12} & 0.16\,{\color{darkgray}\footnotesize$\pm$\,0.09} & 0.56\,{\color{darkgray}\footnotesize$\pm$\,0.13} & 0.12\,{\color{darkgray}\footnotesize$\pm$\,0.09} & 0.12\,{\color{darkgray}\footnotesize$\pm$\,0.08} & 0.04\,{\color{darkgray}\footnotesize$\pm$\,0.05} & 0.38\,{\color{darkgray}\footnotesize$\pm$\,0.12} & 0.08\,{\color{darkgray}\footnotesize$\pm$\,0.09} & 0.02\,{\color{darkgray}\footnotesize$\pm$\,0.03} \\
\midrule
\multirow{0}{*}{\makecell[l]{Find Extrema }}& Length & 0.99\,{\color{darkgray}\footnotesize$\pm$\,0.02} & 0.97\,{\color{darkgray}\footnotesize$\pm$\,0.03} & 0.97\,{\color{darkgray}\footnotesize$\pm$\,0.03} & 1.00\,{\color{darkgray}\footnotesize$\pm$\,0.00} & 1.00\,{\color{darkgray}\footnotesize$\pm$\,0.00} & 0.98\,{\color{darkgray}\footnotesize$\pm$\,0.02} & 0.99\,{\color{darkgray}\footnotesize$\pm$\,0.02} & 1.00\,{\color{darkgray}\footnotesize$\pm$\,0.00} & 0.40\,{\color{darkgray}\footnotesize$\pm$\,0.10} \\
& Position & 0.93\,{\color{darkgray}\footnotesize$\pm$\,0.06} & 0.69\,{\color{darkgray}\footnotesize$\pm$\,0.08} & 0.97\,{\color{darkgray}\footnotesize$\pm$\,0.03} & 0.83\,{\color{darkgray}\footnotesize$\pm$\,0.07} & 0.84\,{\color{darkgray}\footnotesize$\pm$\,0.07} & 0.66\,{\color{darkgray}\footnotesize$\pm$\,0.08} & 0.93\,{\color{darkgray}\footnotesize$\pm$\,0.05} & 0.98\,{\color{darkgray}\footnotesize$\pm$\,0.03} & 0.25\,{\color{darkgray}\footnotesize$\pm$\,0.08} \\
& Area & 0.96\,{\color{darkgray}\footnotesize$\pm$\,0.03} & 0.88\,{\color{darkgray}\footnotesize$\pm$\,0.06} & 0.98\,{\color{darkgray}\footnotesize$\pm$\,0.03} & 0.85\,{\color{darkgray}\footnotesize$\pm$\,0.05} & 0.87\,{\color{darkgray}\footnotesize$\pm$\,0.06} & 0.80\,{\color{darkgray}\footnotesize$\pm$\,0.07} & 0.88\,{\color{darkgray}\footnotesize$\pm$\,0.06} & 0.97\,{\color{darkgray}\footnotesize$\pm$\,0.03} & 0.34\,{\color{darkgray}\footnotesize$\pm$\,0.09} \\
& Color Quantitative & 1.00\,{\color{darkgray}\footnotesize$\pm$\,0.00} & 0.98\,{\color{darkgray}\footnotesize$\pm$\,0.03} & 1.00\,{\color{darkgray}\footnotesize$\pm$\,0.00} & 0.72\,{\color{darkgray}\footnotesize$\pm$\,0.12} & 0.80\,{\color{darkgray}\footnotesize$\pm$\,0.12} & 0.66\,{\color{darkgray}\footnotesize$\pm$\,0.13} & 0.70\,{\color{darkgray}\footnotesize$\pm$\,0.09} & 0.98\,{\color{darkgray}\footnotesize$\pm$\,0.03} & 0.26\,{\color{darkgray}\footnotesize$\pm$\,0.15} \\
& Color Nominal & 0.98\,{\color{darkgray}\footnotesize$\pm$\,0.02} & 0.92\,{\color{darkgray}\footnotesize$\pm$\,0.07} & 1.00\,{\color{darkgray}\footnotesize$\pm$\,0.00} & 0.66\,{\color{darkgray}\footnotesize$\pm$\,0.12} & 0.50\,{\color{darkgray}\footnotesize$\pm$\,0.11} & 0.38\,{\color{darkgray}\footnotesize$\pm$\,0.13} & 0.72\,{\color{darkgray}\footnotesize$\pm$\,0.12} & 0.50\,{\color{darkgray}\footnotesize$\pm$\,0.12} & 0.12\,{\color{darkgray}\footnotesize$\pm$\,0.09} \\
& Shape & 0.96\,{\color{darkgray}\footnotesize$\pm$\,0.05} & 0.72\,{\color{darkgray}\footnotesize$\pm$\,0.12} & 0.92\,{\color{darkgray}\footnotesize$\pm$\,0.08} & 0.60\,{\color{darkgray}\footnotesize$\pm$\,0.11} & 0.52\,{\color{darkgray}\footnotesize$\pm$\,0.13} & 0.26\,{\color{darkgray}\footnotesize$\pm$\,0.14} & 0.64\,{\color{darkgray}\footnotesize$\pm$\,0.13} & 0.46\,{\color{darkgray}\footnotesize$\pm$\,0.13} & 0.16\,{\color{darkgray}\footnotesize$\pm$\,0.08} \\
\midrule
\multirow{0}{*}{\makecell[l]{Find Anomaly }}& Length & 0.96\,{\color{darkgray}\footnotesize$\pm$\,0.03} & 0.89\,{\color{darkgray}\footnotesize$\pm$\,0.06} & 0.96\,{\color{darkgray}\footnotesize$\pm$\,0.03} & 0.79\,{\color{darkgray}\footnotesize$\pm$\,0.05} & 0.79\,{\color{darkgray}\footnotesize$\pm$\,0.09} & 0.91\,{\color{darkgray}\footnotesize$\pm$\,0.04} & 0.85\,{\color{darkgray}\footnotesize$\pm$\,0.06} & 0.81\,{\color{darkgray}\footnotesize$\pm$\,0.07} & 0.32\,{\color{darkgray}\footnotesize$\pm$\,0.09} \\
& Position & 0.88\,{\color{darkgray}\footnotesize$\pm$\,0.06} & 0.49\,{\color{darkgray}\footnotesize$\pm$\,0.08} & 0.95\,{\color{darkgray}\footnotesize$\pm$\,0.04} & 0.71\,{\color{darkgray}\footnotesize$\pm$\,0.09} & 0.68\,{\color{darkgray}\footnotesize$\pm$\,0.07} & 0.50\,{\color{darkgray}\footnotesize$\pm$\,0.08} & 0.91\,{\color{darkgray}\footnotesize$\pm$\,0.05} & 0.89\,{\color{darkgray}\footnotesize$\pm$\,0.04} & 0.23\,{\color{darkgray}\footnotesize$\pm$\,0.08} \\
& Area & 0.85\,{\color{darkgray}\footnotesize$\pm$\,0.07} & 0.80\,{\color{darkgray}\footnotesize$\pm$\,0.09} & 0.93\,{\color{darkgray}\footnotesize$\pm$\,0.04} & 0.98\,{\color{darkgray}\footnotesize$\pm$\,0.03} & 0.79\,{\color{darkgray}\footnotesize$\pm$\,0.07} & 0.56\,{\color{darkgray}\footnotesize$\pm$\,0.09} & 0.96\,{\color{darkgray}\footnotesize$\pm$\,0.03} & 0.66\,{\color{darkgray}\footnotesize$\pm$\,0.08} & 0.26\,{\color{darkgray}\footnotesize$\pm$\,0.09} \\
& Color Quantitative & 0.98\,{\color{darkgray}\footnotesize$\pm$\,0.03} & 0.98\,{\color{darkgray}\footnotesize$\pm$\,0.03} & 0.98\,{\color{darkgray}\footnotesize$\pm$\,0.03} & 0.76\,{\color{darkgray}\footnotesize$\pm$\,0.11} & 0.86\,{\color{darkgray}\footnotesize$\pm$\,0.08} & 0.60\,{\color{darkgray}\footnotesize$\pm$\,0.12} & 0.90\,{\color{darkgray}\footnotesize$\pm$\,0.07} & 0.84\,{\color{darkgray}\footnotesize$\pm$\,0.11} & 0.22\,{\color{darkgray}\footnotesize$\pm$\,0.10} \\
& Color Nominal & 0.50\,{\color{darkgray}\footnotesize$\pm$\,0.12} & 0.50\,{\color{darkgray}\footnotesize$\pm$\,0.13} & 0.56\,{\color{darkgray}\footnotesize$\pm$\,0.13} & 0.50\,{\color{darkgray}\footnotesize$\pm$\,0.14} & 0.48\,{\color{darkgray}\footnotesize$\pm$\,0.12} & 0.32\,{\color{darkgray}\footnotesize$\pm$\,0.12} & 0.50\,{\color{darkgray}\footnotesize$\pm$\,0.13} & 0.24\,{\color{darkgray}\footnotesize$\pm$\,0.11} & 0.18\,{\color{darkgray}\footnotesize$\pm$\,0.11} \\
& Shape & 0.50\,{\color{darkgray}\footnotesize$\pm$\,0.12} & 0.46\,{\color{darkgray}\footnotesize$\pm$\,0.11} & 0.62\,{\color{darkgray}\footnotesize$\pm$\,0.15} & 0.50\,{\color{darkgray}\footnotesize$\pm$\,0.13} & 0.34\,{\color{darkgray}\footnotesize$\pm$\,0.12} & 0.38\,{\color{darkgray}\footnotesize$\pm$\,0.11} & 0.48\,{\color{darkgray}\footnotesize$\pm$\,0.14} & 0.44\,{\color{darkgray}\footnotesize$\pm$\,0.12} & 0.20\,{\color{darkgray}\footnotesize$\pm$\,0.09} \\
\midrule
\multirow{0}{*}{\makecell[l]{Compute Derived \\ Value Exact }}& Length & 0.40\,{\color{darkgray}\footnotesize$\pm$\,0.14} & 0.28\,{\color{darkgray}\footnotesize$\pm$\,0.13} & 0.32\,{\color{darkgray}\footnotesize$\pm$\,0.12} & 0.24\,{\color{darkgray}\footnotesize$\pm$\,0.13} & 0.30\,{\color{darkgray}\footnotesize$\pm$\,0.12} & 0.30\,{\color{darkgray}\footnotesize$\pm$\,0.10} & 0.34\,{\color{darkgray}\footnotesize$\pm$\,0.10} & 0.34\,{\color{darkgray}\footnotesize$\pm$\,0.11} & 0.28\,{\color{darkgray}\footnotesize$\pm$\,0.10} \\
& Position & 0.26\,{\color{darkgray}\footnotesize$\pm$\,0.12} & 0.32\,{\color{darkgray}\footnotesize$\pm$\,0.12} & 0.30\,{\color{darkgray}\footnotesize$\pm$\,0.11} & 0.22\,{\color{darkgray}\footnotesize$\pm$\,0.11} & 0.20\,{\color{darkgray}\footnotesize$\pm$\,0.12} & 0.16\,{\color{darkgray}\footnotesize$\pm$\,0.09} & 0.34\,{\color{darkgray}\footnotesize$\pm$\,0.11} & 0.32\,{\color{darkgray}\footnotesize$\pm$\,0.12} & 0.14\,{\color{darkgray}\footnotesize$\pm$\,0.08} \\
& Area & 0.16\,{\color{darkgray}\footnotesize$\pm$\,0.13} & 0.26\,{\color{darkgray}\footnotesize$\pm$\,0.11} & 0.10\,{\color{darkgray}\footnotesize$\pm$\,0.06} & 0.40\,{\color{darkgray}\footnotesize$\pm$\,0.11} & 0.32\,{\color{darkgray}\footnotesize$\pm$\,0.11} & 0.22\,{\color{darkgray}\footnotesize$\pm$\,0.09} & 0.16\,{\color{darkgray}\footnotesize$\pm$\,0.10} & 0.22\,{\color{darkgray}\footnotesize$\pm$\,0.12} & 0.00\,{\color{darkgray}\footnotesize$\pm$\,0.00} \\
& Color Quantitative & 0.16\,{\color{darkgray}\footnotesize$\pm$\,0.14} & 0.12\,{\color{darkgray}\footnotesize$\pm$\,0.12} & 0.16\,{\color{darkgray}\footnotesize$\pm$\,0.10} & 0.12\,{\color{darkgray}\footnotesize$\pm$\,0.12} & 0.20\,{\color{darkgray}\footnotesize$\pm$\,0.16} & 0.04\,{\color{darkgray}\footnotesize$\pm$\,0.06} & 0.08\,{\color{darkgray}\footnotesize$\pm$\,0.08} & 0.20\,{\color{darkgray}\footnotesize$\pm$\,0.14} & 0.00\,{\color{darkgray}\footnotesize$\pm$\,0.00} \\
& Color Nominal & 0.04\,{\color{darkgray}\footnotesize$\pm$\,0.04} & 0.02\,{\color{darkgray}\footnotesize$\pm$\,0.03} & 0.78\,{\color{darkgray}\footnotesize$\pm$\,0.09} & 0.00\,{\color{darkgray}\footnotesize$\pm$\,0.00} & 0.00\,{\color{darkgray}\footnotesize$\pm$\,0.00} & 0.00\,{\color{darkgray}\footnotesize$\pm$\,0.00} & 0.00\,{\color{darkgray}\footnotesize$\pm$\,0.00} & 0.00\,{\color{darkgray}\footnotesize$\pm$\,0.00} & 0.00\,{\color{darkgray}\footnotesize$\pm$\,0.00} \\
& Shape & 0.00\,{\color{darkgray}\footnotesize$\pm$\,0.00} & 0.02\,{\color{darkgray}\footnotesize$\pm$\,0.04} & 0.56\,{\color{darkgray}\footnotesize$\pm$\,0.11} & 0.00\,{\color{darkgray}\footnotesize$\pm$\,0.00} & 0.00\,{\color{darkgray}\footnotesize$\pm$\,0.00} & 0.00\,{\color{darkgray}\footnotesize$\pm$\,0.00} & 0.00\,{\color{darkgray}\footnotesize$\pm$\,0.00} & 0.00\,{\color{darkgray}\footnotesize$\pm$\,0.00} & 0.00\,{\color{darkgray}\footnotesize$\pm$\,0.00} \\
\midrule
\multirow{0}{*}{\makecell[l]{Compute Derived \\ Value Relative }}& Length & 0.98\,{\color{darkgray}\footnotesize$\pm$\,0.03} & 0.66\,{\color{darkgray}\footnotesize$\pm$\,0.10} & 1.00\,{\color{darkgray}\footnotesize$\pm$\,0.00} & 0.80\,{\color{darkgray}\footnotesize$\pm$\,0.11} & 0.76\,{\color{darkgray}\footnotesize$\pm$\,0.07} & 0.58\,{\color{darkgray}\footnotesize$\pm$\,0.10} & 0.78\,{\color{darkgray}\footnotesize$\pm$\,0.12} & 0.78\,{\color{darkgray}\footnotesize$\pm$\,0.11} & 0.66\,{\color{darkgray}\footnotesize$\pm$\,0.14} \\
& Position & 0.70\,{\color{darkgray}\footnotesize$\pm$\,0.13} & 0.64\,{\color{darkgray}\footnotesize$\pm$\,0.12} & 0.70\,{\color{darkgray}\footnotesize$\pm$\,0.11} & 0.68\,{\color{darkgray}\footnotesize$\pm$\,0.10} & 0.68\,{\color{darkgray}\footnotesize$\pm$\,0.14} & 0.36\,{\color{darkgray}\footnotesize$\pm$\,0.12} & 0.64\,{\color{darkgray}\footnotesize$\pm$\,0.12} & 0.68\,{\color{darkgray}\footnotesize$\pm$\,0.12} & 0.20\,{\color{darkgray}\footnotesize$\pm$\,0.10} \\
& Area & 1.00\,{\color{darkgray}\footnotesize$\pm$\,0.00} & 0.92\,{\color{darkgray}\footnotesize$\pm$\,0.08} & 0.98\,{\color{darkgray}\footnotesize$\pm$\,0.03} & 1.00\,{\color{darkgray}\footnotesize$\pm$\,0.00} & 1.00\,{\color{darkgray}\footnotesize$\pm$\,0.00} & 0.48\,{\color{darkgray}\footnotesize$\pm$\,0.15} & 1.00\,{\color{darkgray}\footnotesize$\pm$\,0.00} & 1.00\,{\color{darkgray}\footnotesize$\pm$\,0.00} & 0.58\,{\color{darkgray}\footnotesize$\pm$\,0.13} \\
& Color Quantitative & 1.00\,{\color{darkgray}\footnotesize$\pm$\,0.00} & 1.00\,{\color{darkgray}\footnotesize$\pm$\,0.00} & 1.00\,{\color{darkgray}\footnotesize$\pm$\,0.00} & 1.00\,{\color{darkgray}\footnotesize$\pm$\,0.00} & 1.00\,{\color{darkgray}\footnotesize$\pm$\,0.00} & 0.56\,{\color{darkgray}\footnotesize$\pm$\,0.18} & 1.00\,{\color{darkgray}\footnotesize$\pm$\,0.00} & 1.00\,{\color{darkgray}\footnotesize$\pm$\,0.00} & 0.40\,{\color{darkgray}\footnotesize$\pm$\,0.21} \\
& Color Nominal & 0.64\,{\color{darkgray}\footnotesize$\pm$\,0.18} & 0.36\,{\color{darkgray}\footnotesize$\pm$\,0.18} & 1.00\,{\color{darkgray}\footnotesize$\pm$\,0.00} & 0.44\,{\color{darkgray}\footnotesize$\pm$\,0.18} & 0.76\,{\color{darkgray}\footnotesize$\pm$\,0.18} & 0.64\,{\color{darkgray}\footnotesize$\pm$\,0.18} & 0.44\,{\color{darkgray}\footnotesize$\pm$\,0.22} & 0.28\,{\color{darkgray}\footnotesize$\pm$\,0.17} & 0.40\,{\color{darkgray}\footnotesize$\pm$\,0.16} \\
& Shape & 0.28\,{\color{darkgray}\footnotesize$\pm$\,0.19} & 0.20\,{\color{darkgray}\footnotesize$\pm$\,0.12} & 1.00\,{\color{darkgray}\footnotesize$\pm$\,0.00} & 0.64\,{\color{darkgray}\footnotesize$\pm$\,0.16} & 0.60\,{\color{darkgray}\footnotesize$\pm$\,0.16} & 0.44\,{\color{darkgray}\footnotesize$\pm$\,0.16} & 0.48\,{\color{darkgray}\footnotesize$\pm$\,0.18} & 0.52\,{\color{darkgray}\footnotesize$\pm$\,0.16} & 0.56\,{\color{darkgray}\footnotesize$\pm$\,0.18} \\
\midrule
\multirow{0}{*}{\makecell[l]{Correlate Values }}& Length & 0.51\,{\color{darkgray}\footnotesize$\pm$\,0.09} & 0.56\,{\color{darkgray}\footnotesize$\pm$\,0.09} & 0.71\,{\color{darkgray}\footnotesize$\pm$\,0.08} & 0.54\,{\color{darkgray}\footnotesize$\pm$\,0.09} & 0.57\,{\color{darkgray}\footnotesize$\pm$\,0.10} & 0.61\,{\color{darkgray}\footnotesize$\pm$\,0.09} & 0.58\,{\color{darkgray}\footnotesize$\pm$\,0.09} & 0.50\,{\color{darkgray}\footnotesize$\pm$\,0.09} & 0.34\,{\color{darkgray}\footnotesize$\pm$\,0.08} \\
& Position & 0.96\,{\color{darkgray}\footnotesize$\pm$\,0.05} & 0.90\,{\color{darkgray}\footnotesize$\pm$\,0.07} & 0.92\,{\color{darkgray}\footnotesize$\pm$\,0.06} & 0.56\,{\color{darkgray}\footnotesize$\pm$\,0.14} & 0.50\,{\color{darkgray}\footnotesize$\pm$\,0.12} & 0.58\,{\color{darkgray}\footnotesize$\pm$\,0.12} & 0.60\,{\color{darkgray}\footnotesize$\pm$\,0.13} & 0.50\,{\color{darkgray}\footnotesize$\pm$\,0.10} & 0.04\,{\color{darkgray}\footnotesize$\pm$\,0.05} \\
& Area & 0.75\,{\color{darkgray}\footnotesize$\pm$\,0.08} & 0.50\,{\color{darkgray}\footnotesize$\pm$\,0.07} & 0.86\,{\color{darkgray}\footnotesize$\pm$\,0.06} & 0.58\,{\color{darkgray}\footnotesize$\pm$\,0.10} & 0.55\,{\color{darkgray}\footnotesize$\pm$\,0.09} & 0.50\,{\color{darkgray}\footnotesize$\pm$\,0.11} & 0.50\,{\color{darkgray}\footnotesize$\pm$\,0.11} & 0.50\,{\color{darkgray}\footnotesize$\pm$\,0.08} & 0.23\,{\color{darkgray}\footnotesize$\pm$\,0.07} \\
& Color Quantitative & 0.70\,{\color{darkgray}\footnotesize$\pm$\,0.13} & 0.48\,{\color{darkgray}\footnotesize$\pm$\,0.13} & 0.90\,{\color{darkgray}\footnotesize$\pm$\,0.09} & 0.56\,{\color{darkgray}\footnotesize$\pm$\,0.11} & 0.64\,{\color{darkgray}\footnotesize$\pm$\,0.18} & 0.60\,{\color{darkgray}\footnotesize$\pm$\,0.14} & 0.50\,{\color{darkgray}\footnotesize$\pm$\,0.15} & 0.50\,{\color{darkgray}\footnotesize$\pm$\,0.12} & 0.28\,{\color{darkgray}\footnotesize$\pm$\,0.11} \\
\midrule
\multirow{0}{*}{\makecell[l]{Correlate Values \\ Relative }}& Length & 0.82\,{\color{darkgray}\footnotesize$\pm$\,0.09} & 0.54\,{\color{darkgray}\footnotesize$\pm$\,0.13} & 0.76\,{\color{darkgray}\footnotesize$\pm$\,0.14} & 0.60\,{\color{darkgray}\footnotesize$\pm$\,0.12} & 0.52\,{\color{darkgray}\footnotesize$\pm$\,0.11} & 0.52\,{\color{darkgray}\footnotesize$\pm$\,0.13} & 0.62\,{\color{darkgray}\footnotesize$\pm$\,0.11} & 0.52\,{\color{darkgray}\footnotesize$\pm$\,0.12} & 0.44\,{\color{darkgray}\footnotesize$\pm$\,0.11} \\
& Position & 1.00\,{\color{darkgray}\footnotesize$\pm$\,0.00} & 0.96\,{\color{darkgray}\footnotesize$\pm$\,0.06} & 0.96\,{\color{darkgray}\footnotesize$\pm$\,0.06} & 0.68\,{\color{darkgray}\footnotesize$\pm$\,0.15} & 0.52\,{\color{darkgray}\footnotesize$\pm$\,0.18} & 0.44\,{\color{darkgray}\footnotesize$\pm$\,0.17} & 0.88\,{\color{darkgray}\footnotesize$\pm$\,0.16} & 0.64\,{\color{darkgray}\footnotesize$\pm$\,0.18} & 0.48\,{\color{darkgray}\footnotesize$\pm$\,0.16} \\
& Area & 0.52\,{\color{darkgray}\footnotesize$\pm$\,0.15} & 0.32\,{\color{darkgray}\footnotesize$\pm$\,0.08} & 0.74\,{\color{darkgray}\footnotesize$\pm$\,0.13} & 0.58\,{\color{darkgray}\footnotesize$\pm$\,0.13} & 0.50\,{\color{darkgray}\footnotesize$\pm$\,0.14} & 0.54\,{\color{darkgray}\footnotesize$\pm$\,0.13} & 0.48\,{\color{darkgray}\footnotesize$\pm$\,0.12} & 0.44\,{\color{darkgray}\footnotesize$\pm$\,0.11} & 0.42\,{\color{darkgray}\footnotesize$\pm$\,0.13} \\
& Color Quantitative & 0.56\,{\color{darkgray}\footnotesize$\pm$\,0.16} & 0.40\,{\color{darkgray}\footnotesize$\pm$\,0.16} & 0.84\,{\color{darkgray}\footnotesize$\pm$\,0.12} & 0.72\,{\color{darkgray}\footnotesize$\pm$\,0.12} & 0.68\,{\color{darkgray}\footnotesize$\pm$\,0.16} & 0.72\,{\color{darkgray}\footnotesize$\pm$\,0.16} & 0.28\,{\color{darkgray}\footnotesize$\pm$\,0.14} & 0.36\,{\color{darkgray}\footnotesize$\pm$\,0.16} & 0.48\,{\color{darkgray}\footnotesize$\pm$\,0.18} \\
\bottomrule
\end{tabular}
\end{table}
% \clearpage % ensures the page ends here
% \pagestyle{plain} % reset to default after this page
\end{landscape}
